# Supplementary material for: Object-centric Video Representation for Long-term Action Anticipation
Source: arXiv:2311.00180 source file (2023-10-31)
Supplement: Supplementary file 1 [file Appendix_Object_attention_rollout_heatmap.pdf]

$Z = 0$

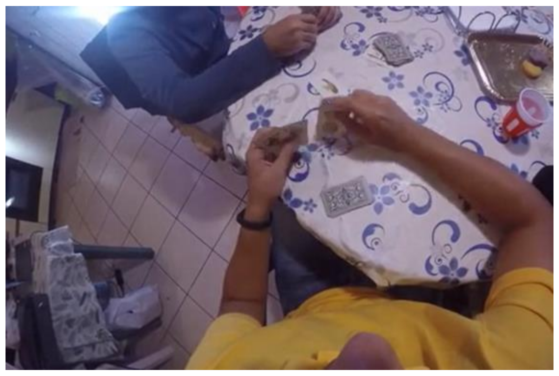

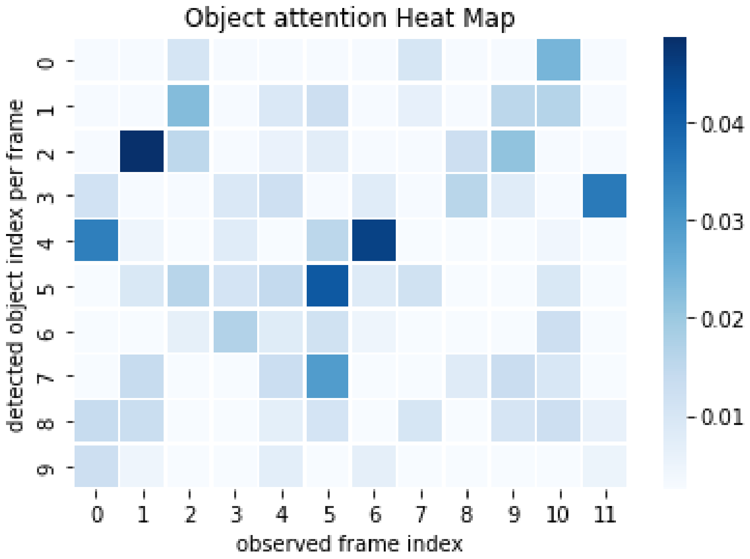


$(v_{gt}, n_{gt})$ = (take, card)

Top 3 weighted objects from Attention Map at **6$^{th}$ frame**: ['card', 'paper', 'container']

$Z = 5$

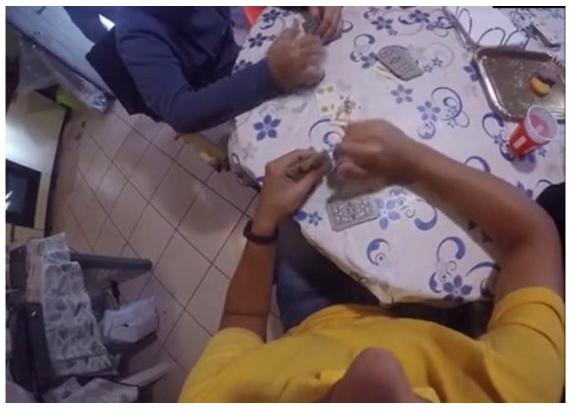

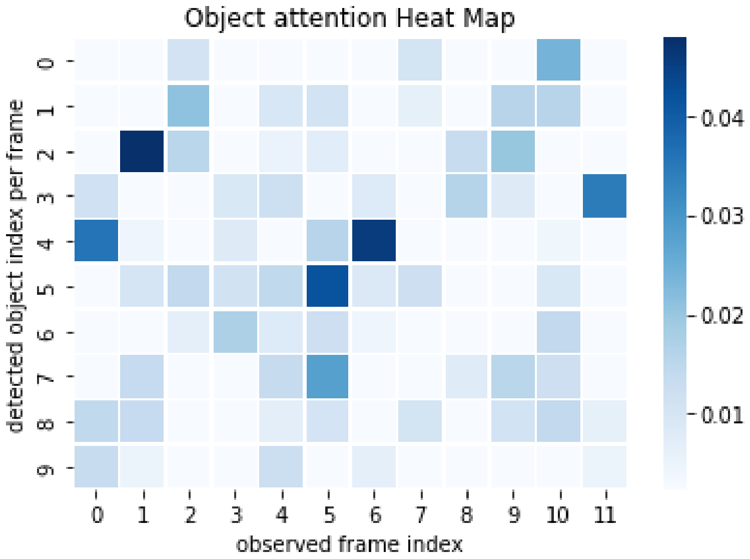


$(v_{gt}, n_{gt})$ = (put, card)

Top 3 weighted objects from Attention Map at **6$^{th}$ frame**: ['card', 'container', 'paper']

$Z = 10$

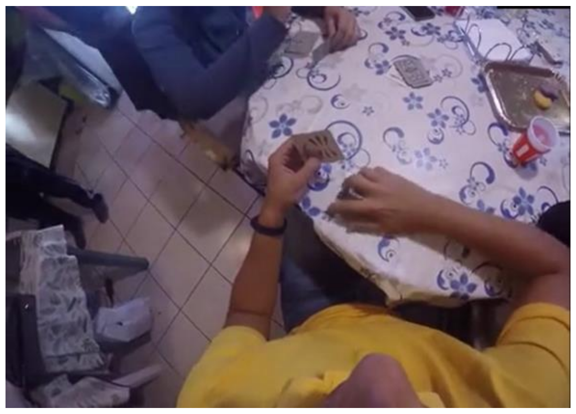

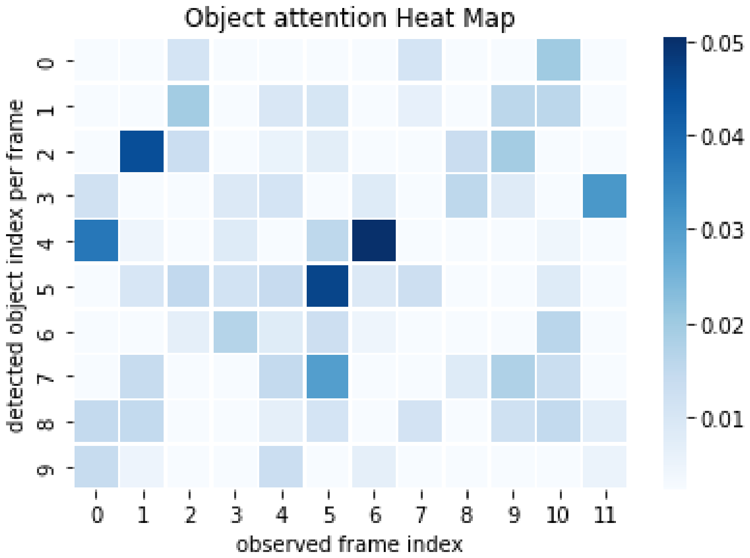


$(v_{gt}, n_{gt})$ = (put, card)

Top 3 weighted objects from Attention Map at **6$^{th}$ frame**: ['card', 'paper', 'container']

$Z = 15$

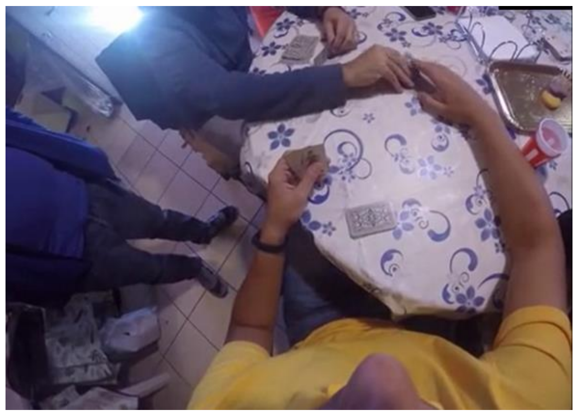

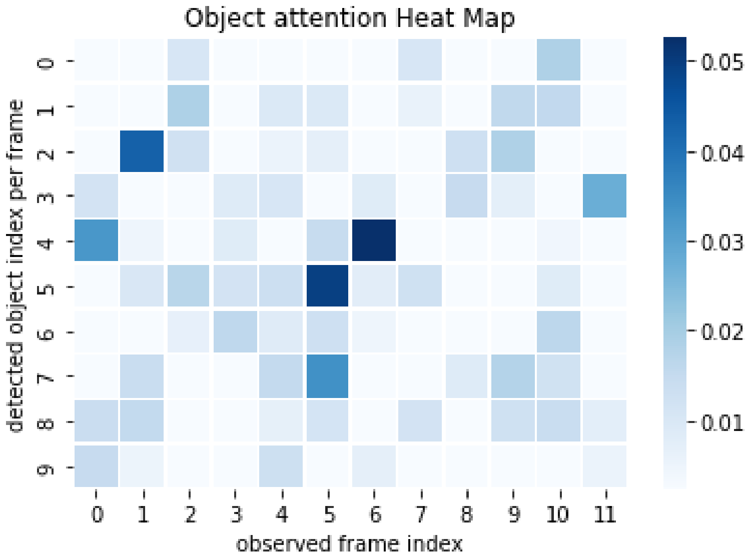


$(v_{gt}, n_{gt})$ = (put, card)

Top 3 weighted objects from Attention Map at **6$^{th}$ frame**: ['card', 'paper', 'container']

$Z = 0$

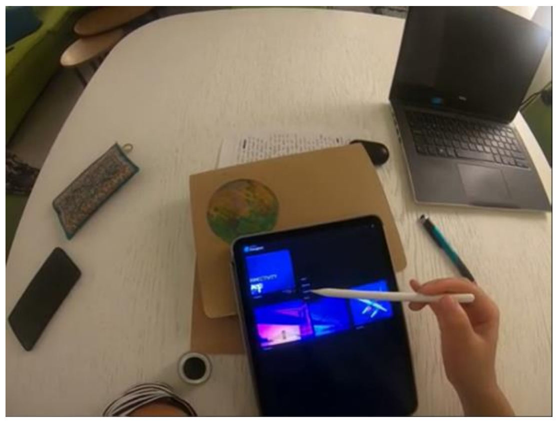

$(v_{gt}, n_{gt})$ = (adjust, pen)

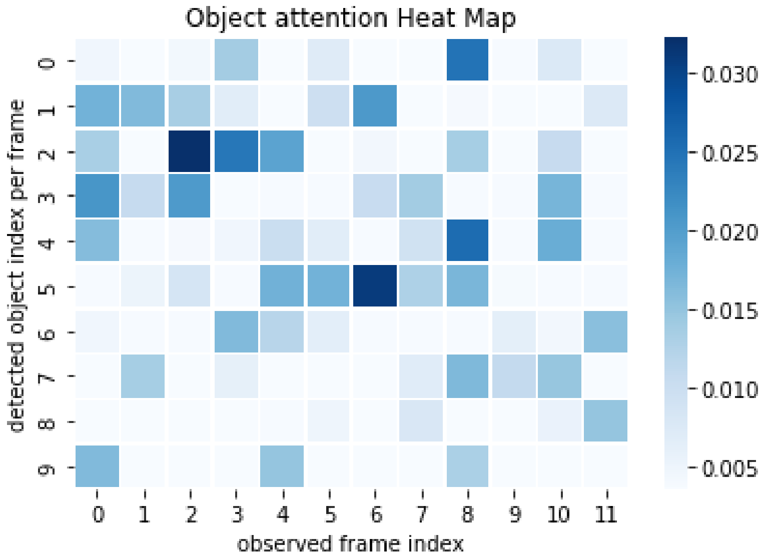


Top 3 weighted objects from Attention Map at **6$^{th}$ frame**: ['computer', 'pencil', 'shoe']

$Z = 5$

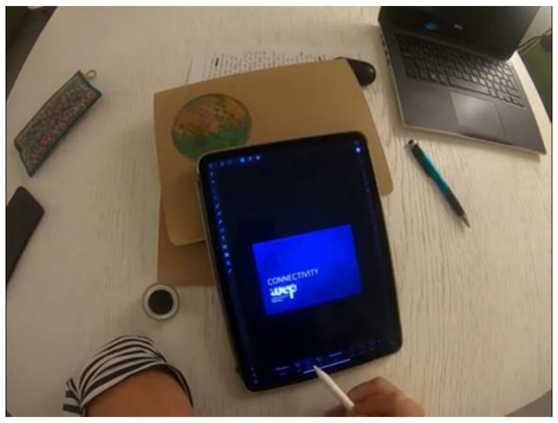

$(v_{gt}, n_{gt})$ = (operate, tablet)

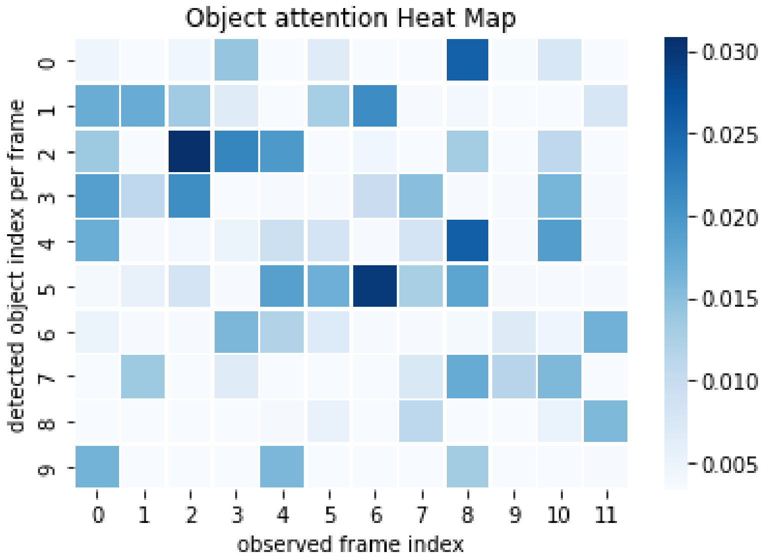


Top 3 weighted objects from Attention Map at **6$^{th}$ frame**: ['computer', 'pencil', 'tablet']

$Z = 10$

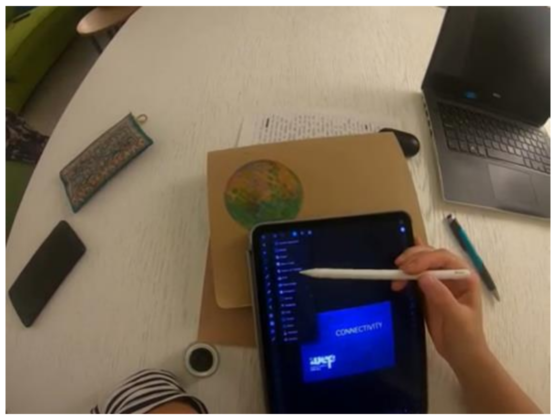

$(v_{gt}, n_{gt})$ = (move, pen)

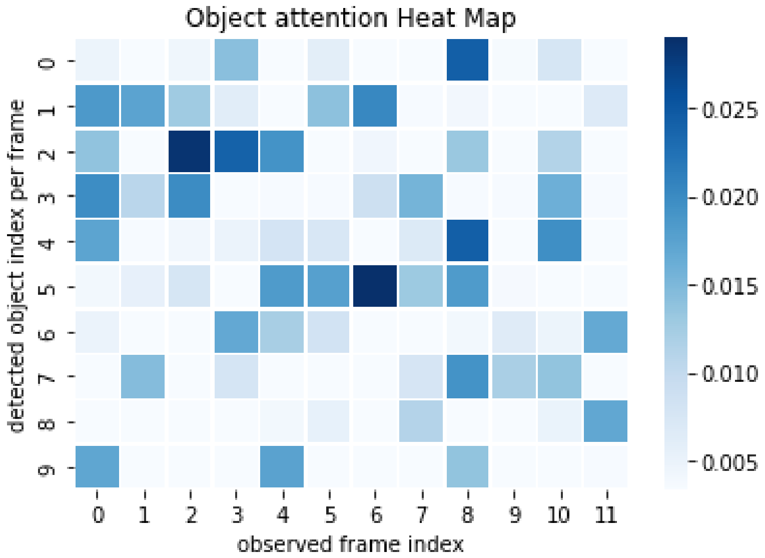


Top 3 weighted objects from Attention Map at **6$^{th}$ frame**: ['computer', 'tablet', 'pencil']

$Z = 15$

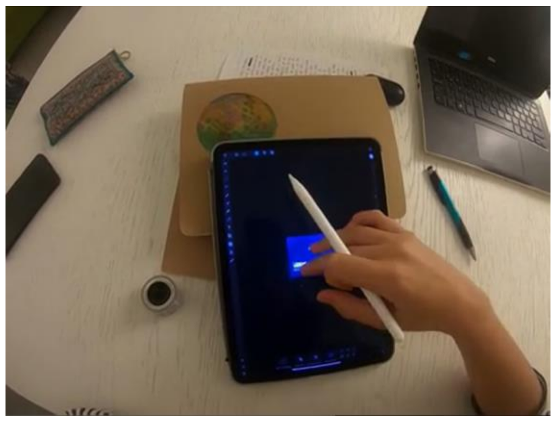

$(v_{gt}, n_{gt})$ = (operate, tablet)

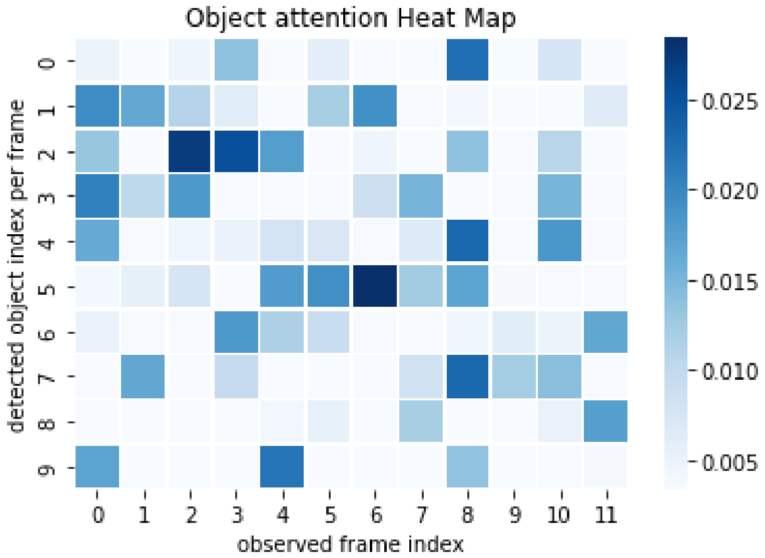


Top 3 weighted objects from Attention Map at **6$^{th}$ frame**: ['computer', 'pencil', 'tablet ']

$Z = 0$

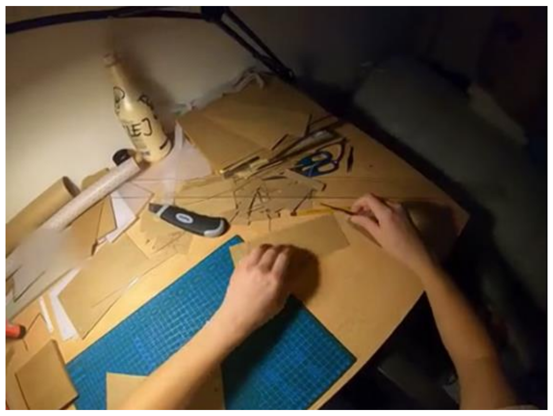

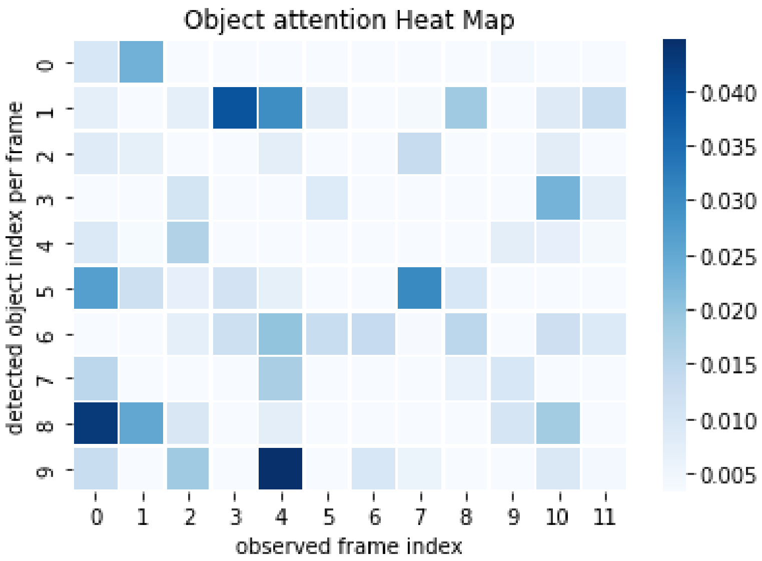


$(v_{gt}, n_{gt})$ = (put, paper)

Top 3 weighted objects from Attention Map at **$6^{th}$ frame**: ['ruler', 'handle', 'paper']

$Z = 5$

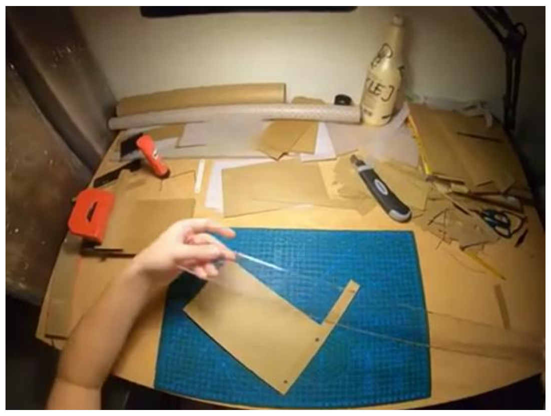

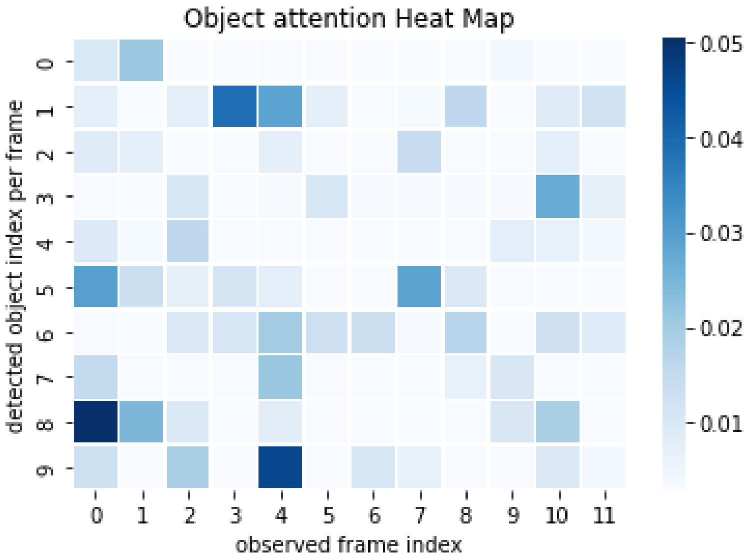


$(v_{gt}, n_{gt})$ = (adjust, ruler)

Top 3 weighted objects from Attention Map at **$6^{th}$ frame**: ['handle', 'ruler', 'container']

$Z = 10$

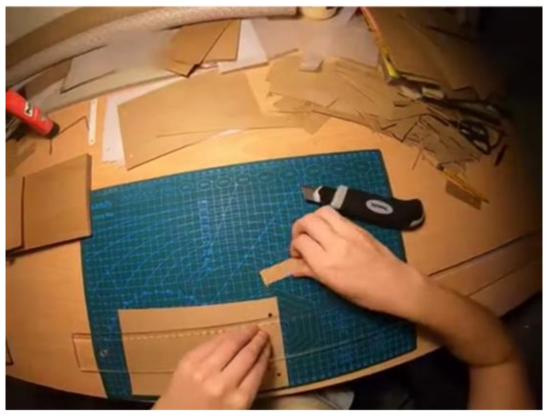

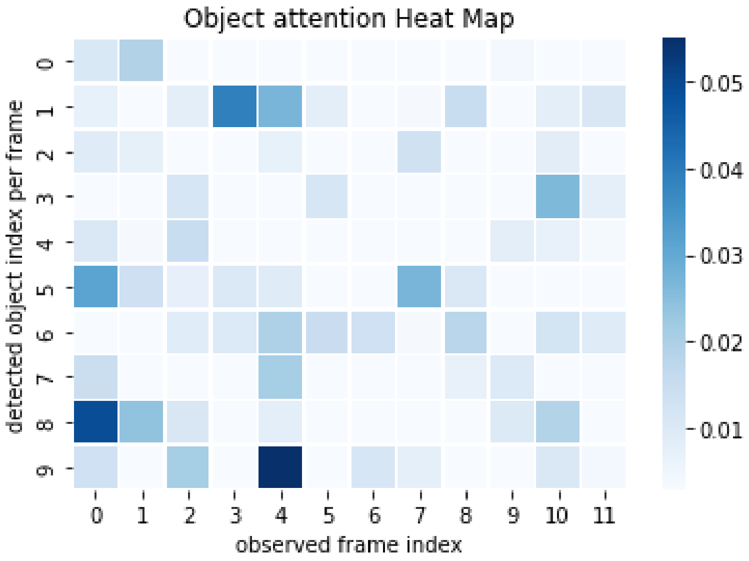


$(v_{gt}, n_{gt})$ = (take, paper)

Top 3 weighted objects from Attention Map at **$6^{th}$ frame**: ['handle', 'ruler', 'paper']

$Z = 15$

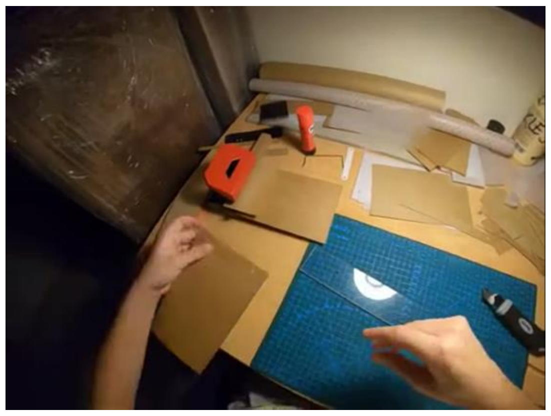

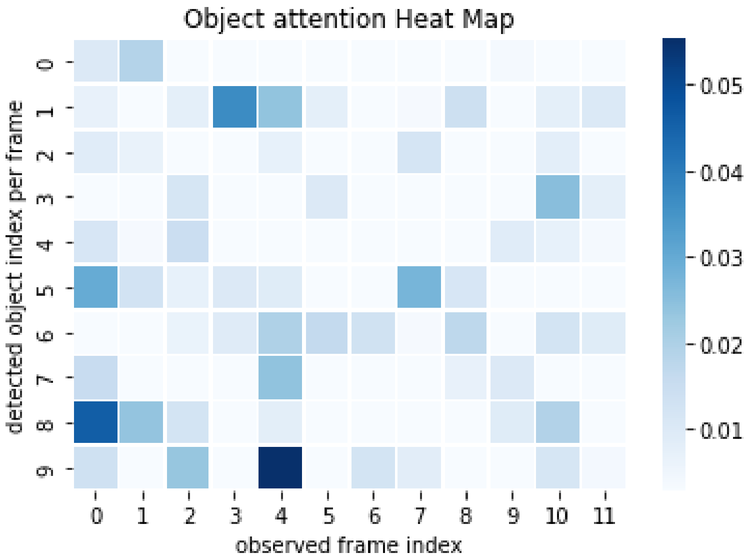


$(v_{gt}, n_{gt})$ = (take, paper)

Top 3 weighted objects from Attention Map at **$6^{th}$ frame**: ['handle', 'ruler', 'paper']

$Z = 0$

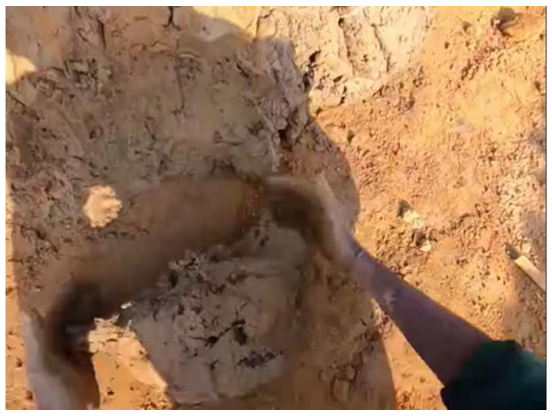

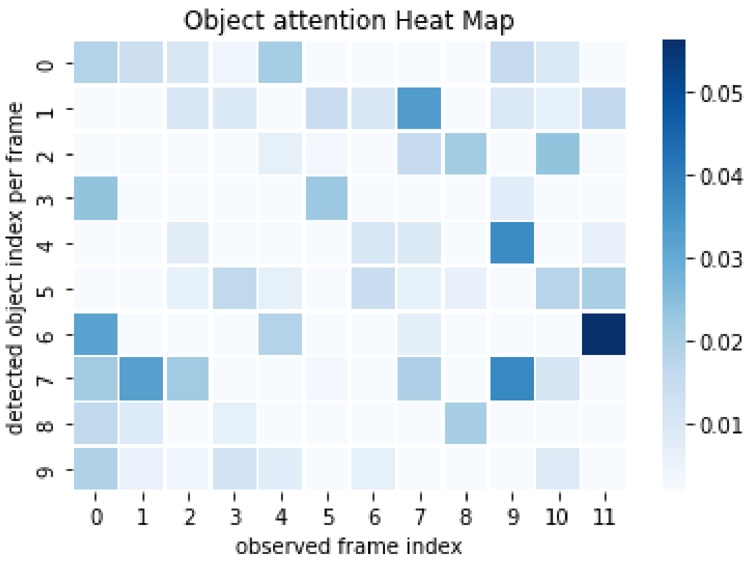


$(v_{gt}, n_{gt})$ = (move, mold)

Top 3 weighted objects from Attention Map at $\mathbf{6^{th}}$ **frame**: ['mold', 'dog', 'clay']

$Z = 5$

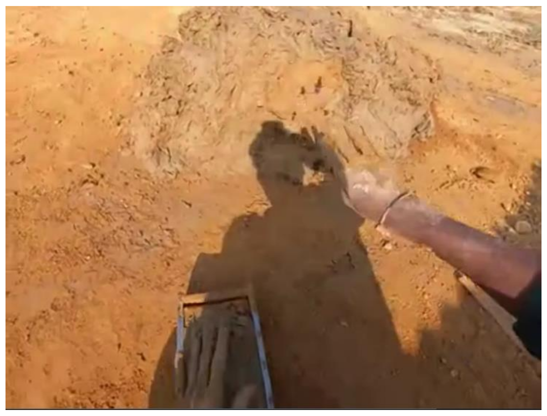

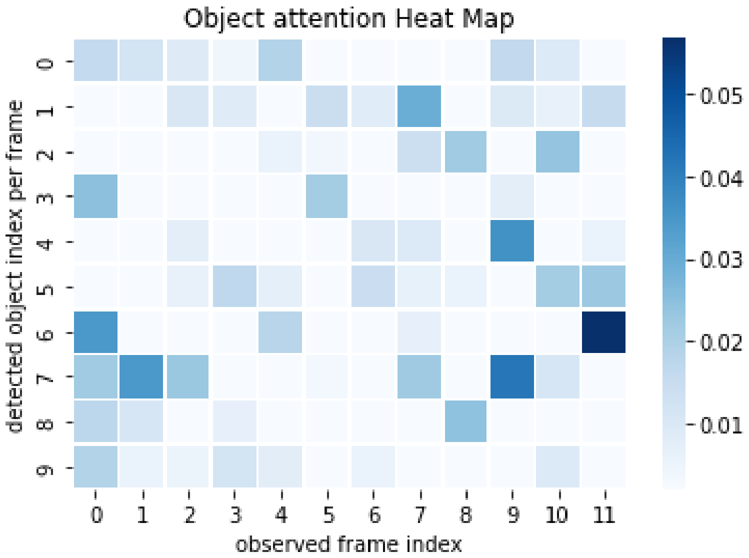


$(v_{gt}, n_{gt})$ = (move, mold)

Top 3 weighted objects from Attention Map at $\mathbf{6^{th}}$ **frame**: ['mold', 'dog', 'clay']

$Z = 10$

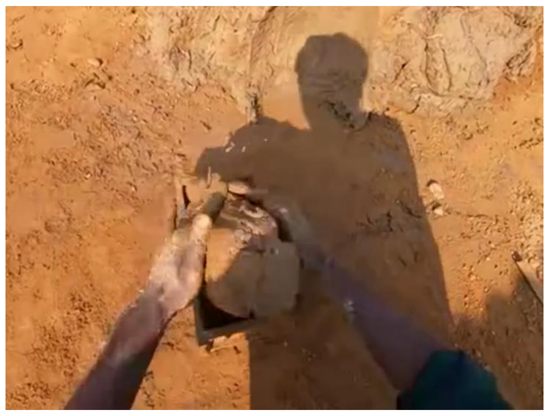

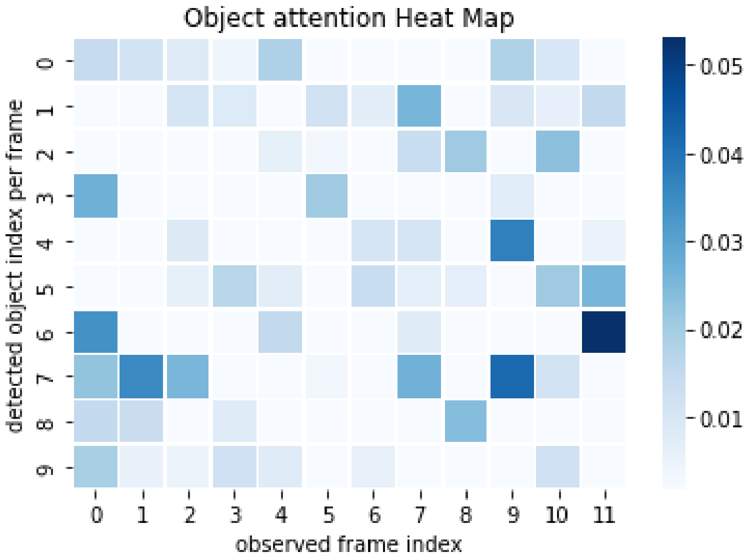


$(v_{gt}, n_{gt})$ = (put, mold)

Top 3 weighted objects from Attention Map at $\mathbf{6^{th}}$ **frame**: ['mold', 'dog', 'clay']

$Z = 15$

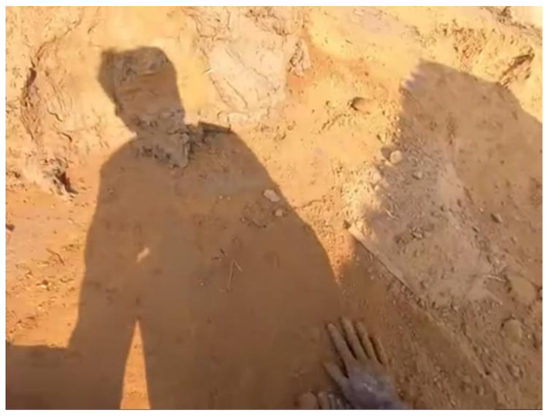

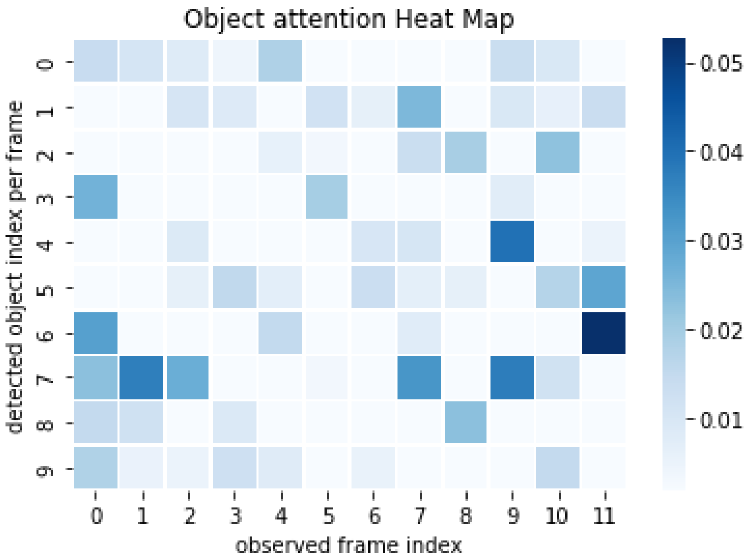


$(v_{gt}, n_{gt})$ = (remove, clay)

Top 3 weighted objects from Attention Map at $\mathbf{6^{th}}$ **frame**: ['mold', 'dog', 'clay']

$Z = 0$

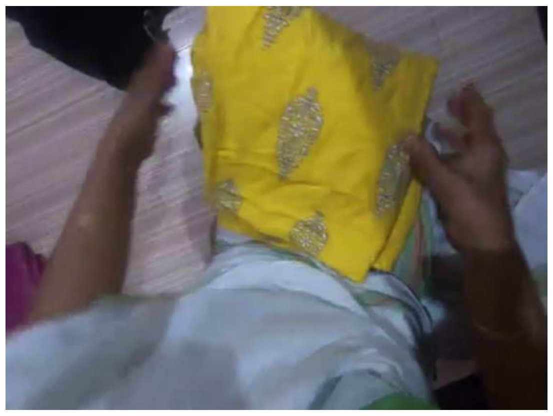

$(v_{gt}, n_{gt})$ = (fold, cloth)

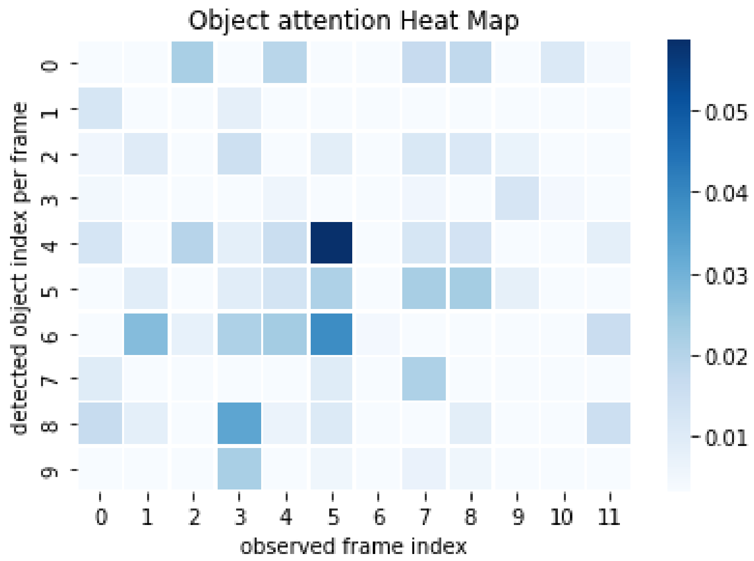


Top 3 weighted objects from Attention Map at **6** $^{th}$ **frame**: ['cloth', 'bag', 'food']

$Z = 5$

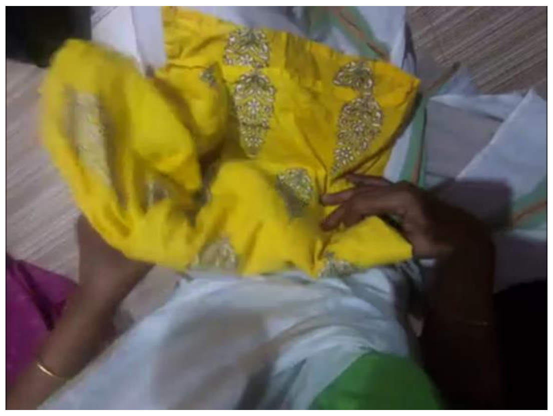

$(v_{gt}, n_{gt})$ = (arrange, cloth)

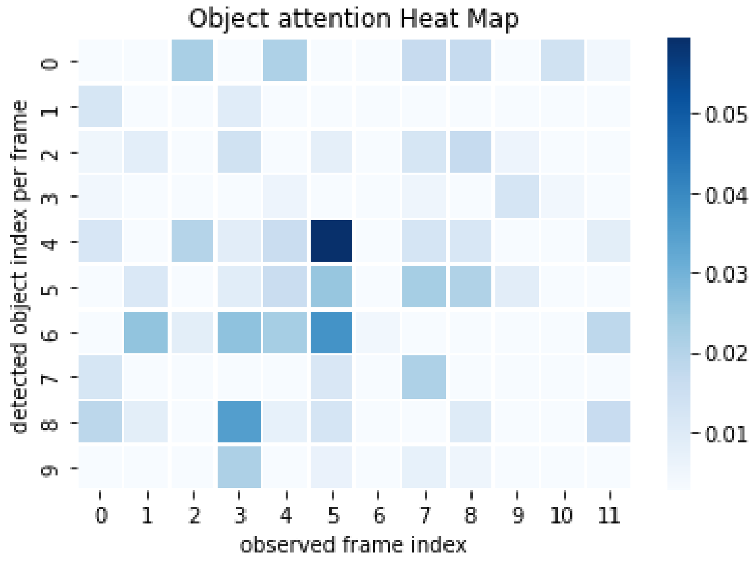


Top 3 weighted objects from Attention Map at **6** $^{th}$ **frame**: ['food', 'bag', 'cloth']

$Z = 10$

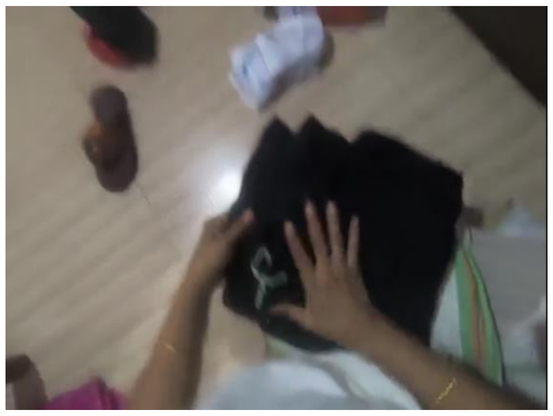

$(v_{gt}, n_{gt})$ = (put, cloth)

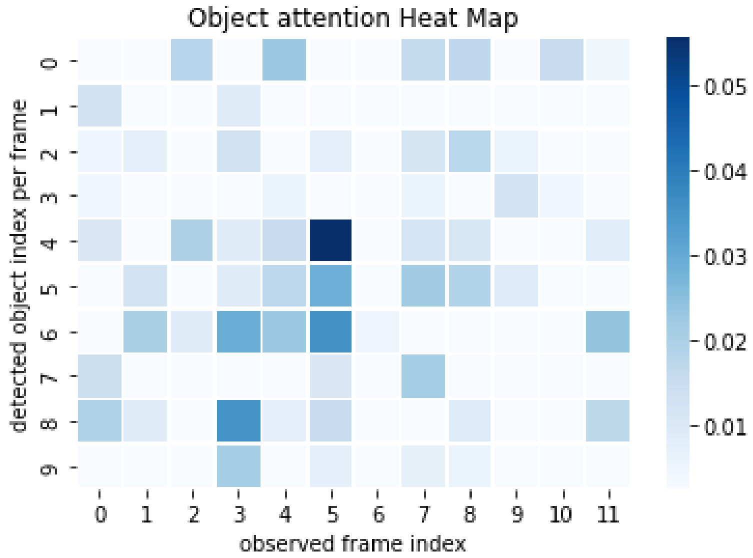


Top 3 weighted objects from Attention Map at **6** $^{th}$ **frame**: ['food', 'bag', 'cloth']

$Z = 15$

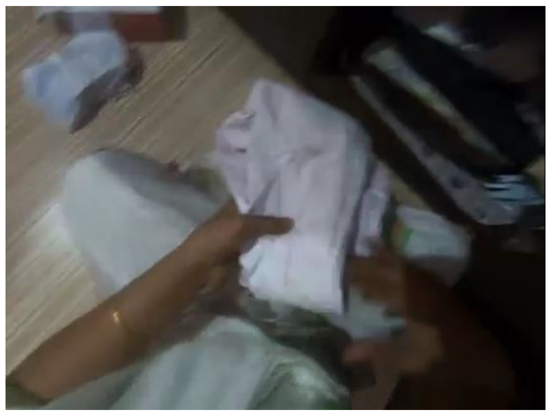

$(v_{gt}, n_{gt})$ = (put, cloth)

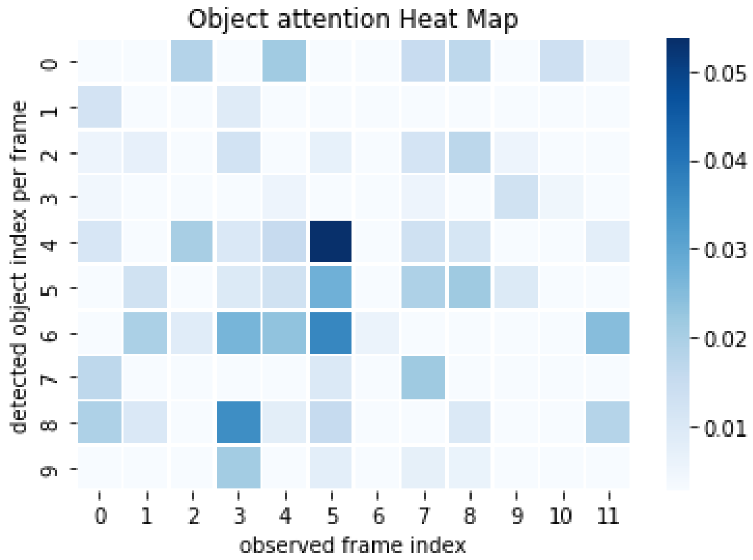


Top 3 weighted objects from Attention Map at **6** $^{th}$ **frame**: ['food', 'cloth', 'bag']

$Z = 0$

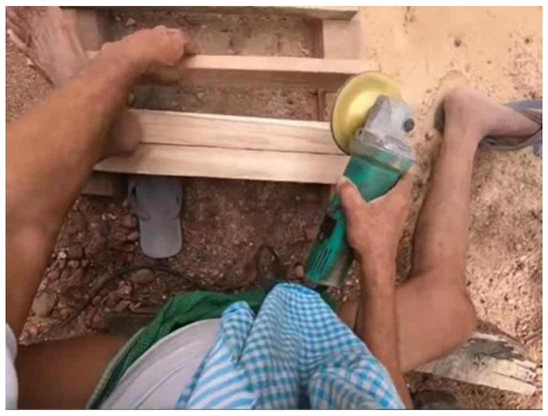

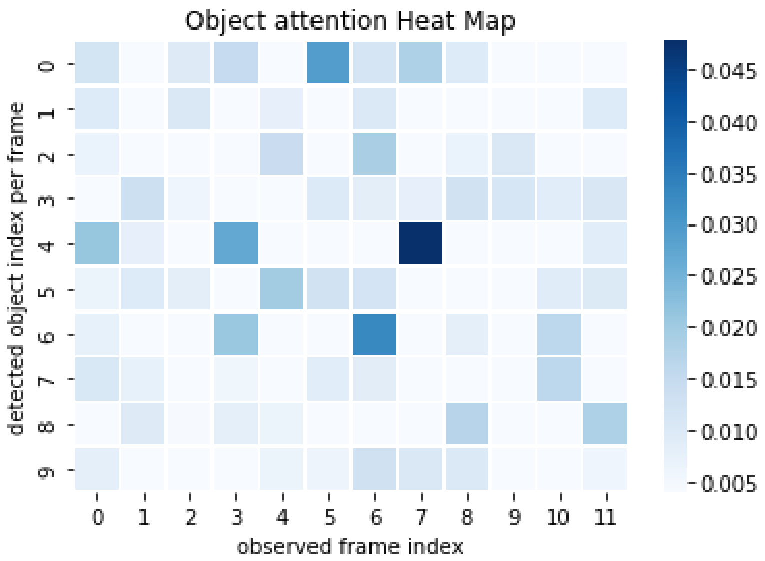


$(v_{gt}, n_{gt})$ = (put, wood)

Top 3 weighted objects from Attention Map at **6$^{th}$ frame**: ['string', 'wood', 'table']

$Z = 5$

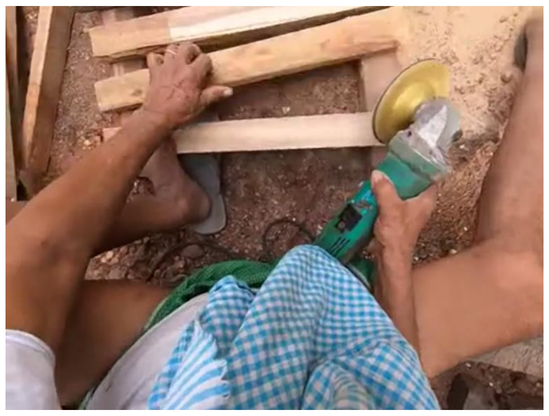

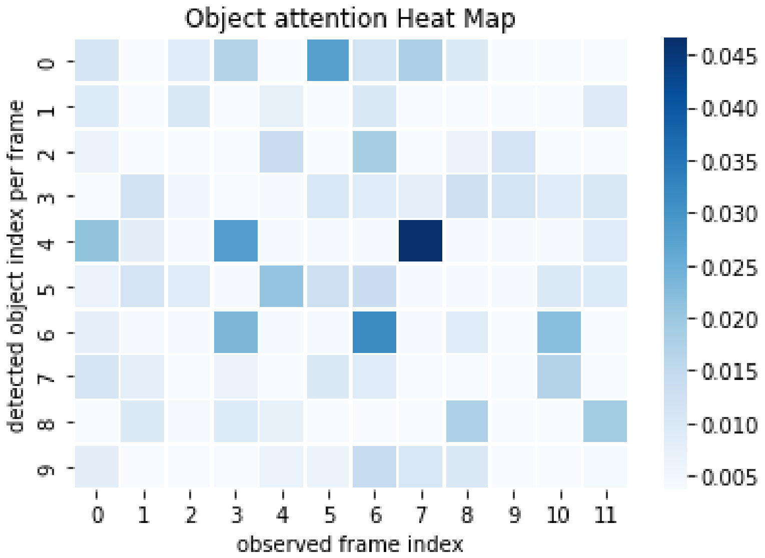


$(v_{gt}, n_{gt})$ = (turn, wood)

Top 3 weighted objects from Attention Map at **6$^{th}$ frame**: ['string', 'table', 'wood']

$Z = 10$

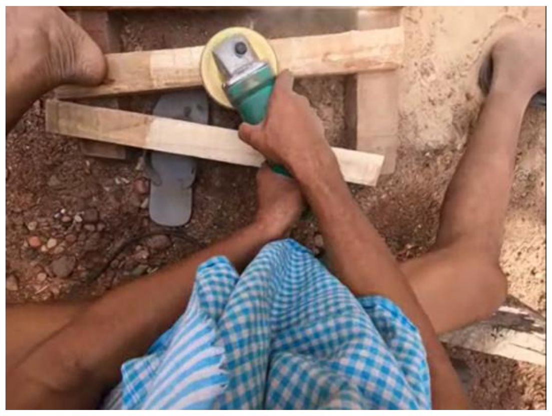

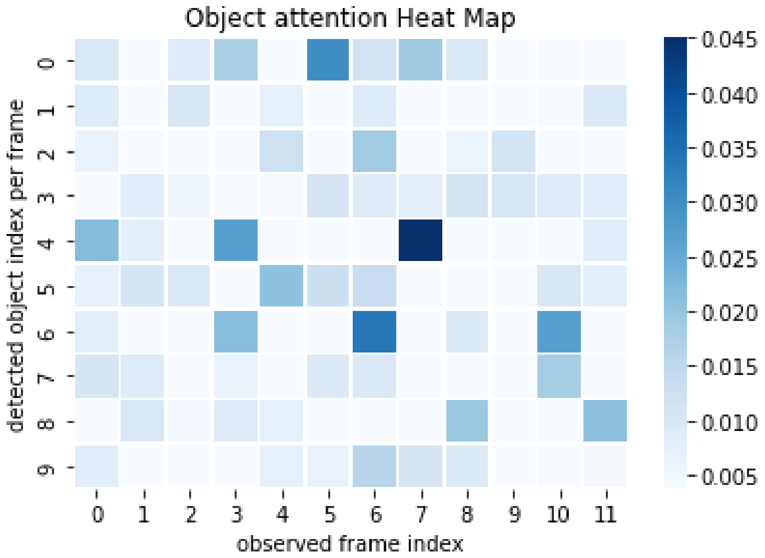


$(v_{gt}, n_{gt})$ = (smooth, wood)

Top 3 weighted objects from Attention Map at **6$^{th}$ frame**: ['string', 'table', 'wood']

$Z = 15$

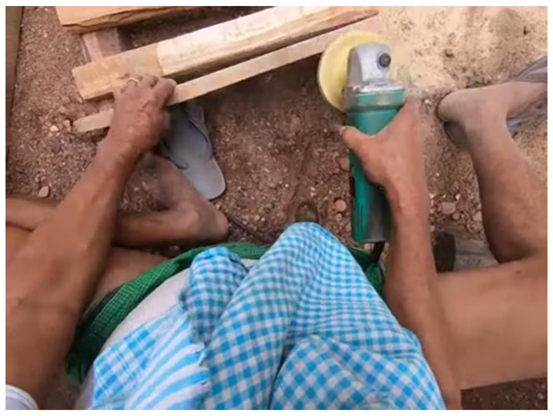

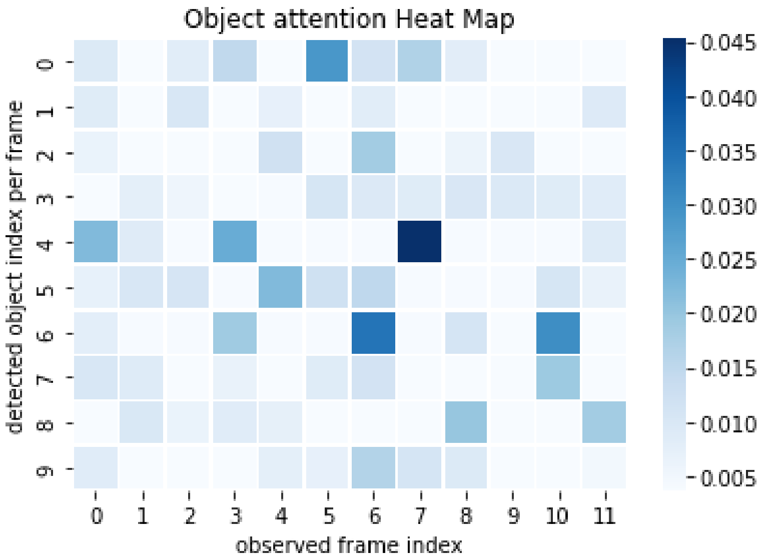


$(v_{gt}, n_{gt})$ = (turn, wood)

Top 3 weighted objects from Attention Map at **6$^{th}$ frame**: ['string', 'table', 'wood']
